# Supplementary material for: Detect, Reject, Correct: Crossmodal Compensation of Corrupted Sensors
Source: arXiv:2012.00201 source file (2020-12-01)
Supplement: Supplementary file 1 [file 6-appendix.tex]

\clearpage

\newpage
\appendix

\section{Representation Training Details}
    \label{appendix:rep}

    \FloatBarrier
    \begin{table}[h!]
        \caption{Loss Functions}
        \label{tab:rep_loss}
        \begin{center}
        \begin{tabular}{ll}
            \hline

             & Loss Function \\
            \hline
            Optical flow & End point error \\
            Optical flow mask & Binary Cross Entropy \\
            EE Pos & Mean Squared Error \\
            Next Contact & Binary Cross Entropy \\
            Pairing & Binary Cross Entropy \\
            KL & KL Divergence \\
            Modality reconstruction & Mean Squared Error + 0.2 * L1 loss \\
            Modality Reconstruction Mask & Mean Squared Error \\
            Latent distance loss & Mean Squared Error\\
            \hline

        \end{tabular}
        \end{center}
    \end{table}
    
    \FloatBarrier
    The loss functions used to train the multimodal representation can be found in Table \ref{tab:rep_loss}. For models with sampling we use $p=0.4$ in all our experiments.

    \begin{table}[h!]
        \caption{Loss Weights}
        \label{tab:rep_weights}

        \begin{center}
        \begin{tabular}{llll}
            \hline

             & Our model & MFM & Sampled MVAE  \\
            \hline
            Optical flow & 50 & 50  & 50\\
            Optical flow mask & 1 & 1  & 1\\
            EE Pos & 1 & 1  & 1\\
            Next Contact & 1 & 1  & 1\\
            Pairing & 1 & 1  & 1\\
            KL & 0.001 & 0.001  & -\\
            Modality reconstruction & 1 & 1  & 1\\
            Modality Reconstruction Mask & 10 & 10  & 10\\
            Latent distance loss & 1 & 1 & 1\\
            MMD & - & 0.001 & - \\
            Missing & - & 0.001 & - \\
            \hline

        \end{tabular}
        \end{center}
    \end{table}
    
    \FloatBarrier
    The weights of the losses used to train the multimodal representation can be found in Table \ref{tab:rep_weights}

\section{OOD Detection Experiment Details}
    \label{appendix:ood}

    \begin{table}[h!]
        \caption{OOD Experiment Hyperparameters}
        \label{tab:ood_hyper}

        \begin{center}
        \begin{tabular}{ll}
            \hline

             & Hyperparameters \\
            \hline
            Random RGB Image / Depth Occlusion & Box height, width $\in$ [30, 60] pixels \\
            & Occlusion around the robot \\ 
            
            Random Lighting Changes & Increase brightness from $b \in \mathcal{U}(0.8, 1)$ \\
            
            Random RGB Image / Depth Rotations & $10 \leq angle \leq 30$ \\
            Blackout force & blackout time steps = 20 \\ 
            Force noise (var) & $\mathcal{N}(0, var) $ \\
            \hline

        \end{tabular}
        \end{center}
    \end{table}
    
    \FloatBarrier
    The hyperparameters for the OOD experiments can be found in Table \ref{tab:ood_hyper}
    
    \FloatBarrier
    \begin{table}[h!]
        \begin{center}
        \begin{tabular}{ccccccc}
            \hline
             & Our model & Our model + Sampling & MFM & MFM + Sampling & VSD & SD \\
             \hline
            img & 0.96 & 0.91 & 0.99 & 0.99 & 0.98 & 0.98 \\
            depth & 1.00 & 1.00 & 1.00 & 1.00 & 1.00 & 1.00 \\
            frc\_avg & 0.83 & 0.80 & 0.92 & 0.89 & 0.88 & 0.82 \\
            frc\_0 & 0.89 & 0.85 & 0.97 & 0.95 & 0.94 & 0.89 \\
            frc\_1 & 0.91 & 0.90 & 0.97 & 0.94 & 0.96 & 0.90 \\
            frc\_2 & 0.90 & 0.88 & 0.98 & 0.97 & 0.97 & 0.87 \\
            frc\_3 & 0.72 & 0.72 & 0.87 & 0.80 & 0.78 & 0.72 \\
            frc\_4 & 0.74 & 0.72 & 0.90 & 0.84 & 0.80 & 0.75 \\
            frc\_5 & 0.80 & 0.73 & 0.83 & 0.84 & 0.81 & 0.76 \\
            \hline
        \end{tabular}%
        \caption{AUROC on val dataset}
        \label{tab:auroc_full}
        \end{center}
    \end{table}
    
    \FloatBarrier
    The breakdown of the AUROC results can be found in Table \ref{tab:auroc_full}
    
    \FloatBarrier
    \begin{table}[h!]
        \begin{center}
        \begin{tabular}{lllll}
            \hline
             & MFM & SD & VSD & Our Model \\
             \hline
            True Vals & 0.94 &  0.80 &  0.80 &  0.92 \\
            RGB Box Occlusions & 1 & 1 & 1 & 0.98 \\
            RGB Lighting Changes & 0.86 &  0.72 &  0.76 &  0.63 \\
            RGB Rotation &  1 & 1 & 1 & 1 \\
            Depth Box Occlusions & 1 & 0.84 &  0.99 &  0.64 \\
            Depth Rotation &  1 & 1 & 1 & 1 \\
            Blackout Force & 1 & 1 & 1 & 1 \\
            Force Noise 0.5 & 1 & 1 & 1 & 1 \\
            Force Noise 0.25 &  0.92 &  1 & 1 & 0.42 \\
            Force Noise 0.1 & 0.21 &  1 & 1 & 0.10 \\

            \hline
        \end{tabular}%
        \caption{Replace Key Accuracy: Accuracy of models in predicting the correct modality to be OOD.}
        \label{appendix:replace_key}
        \end{center}
    \end{table}

\section{Ablation Studies Results}
    \label{appendix:ablation}

\FloatBarrier
    Table \ref{tab:ablation_auroc} shows the results for OOD detection of our ablative models. 

\FloatBarrier
    \begin{table}[h!]
        \begin{center}
            \begin{tabular}{ccccc}
            \hline
             & Our Model & Gen Only & Forward Dynamics Only & No z\_dist \\
             \hline
            img & 0.96 & 0.98 & 0.17 & 0.96 \\
            depth & 1.00 & 0.98 & 0.00 & 1.00 \\
            frc\_avg & 0.83 & 0.90 & 0.51 & 0.74 \\
            frc\_0 & 0.89 & 0.95 & 0.58 & 0.78 \\
            frc\_1 & 0.91 & 0.95 & 0.56 & 0.89 \\
            frc\_2 & 0.90 & 0.95 & 0.58 & 0.79 \\
            frc\_3 & 0.72 & 0.83 & 0.46 & 0.70 \\
            frc\_4 & 0.74 & 0.86 & 0.43 & 0.65 \\
            frc\_5 & 0.80 & 0.82 & 0.46 & 0.65 \\
            \hline
        \end{tabular}%
        \end{center}
        \caption{AUROC on val dataset}
        \label{tab:ablation_auroc_full}
    \end{table}
